# Supplementary material for: Boosting Biomolecular Switch Efficiency With Quantum Coherence
Source: arXiv:2310.17585 source file (2023-10-26)
Supplement: Supplementary file 1 [file appendix1.tex]

\section{Appendix} \label{sec:appendix}
